# Supplementary material for: D4orm: Multi-Robot Trajectories with Dynamics-aware Diffusion Denoised Deformations
Source: arXiv:2503.12204 source file (2026-09-01)
Supplement: Supplementary file 1 [file obstacles.tex]

\newcommand{\entry}[3]{
  \node[] at (\xsize * #1, #2) {
    \includegraphics[width=0.19\linewidth,height=0.15\linewidth]{images/#3}
  };
}

\begin{figure}[tp]
%\centering
\begin{tikzpicture}
    \tikzmath{
        \xoffs = 1.5;   % add space for text (1st col)
        \ystep = -3.0;  % height of a row
  }
  % First row
  \node[anchor=west] at (0,0) {};
  \node[anchor=west] at (0,0) {{\small 1 Obst.}} ;
  \node[anchor=west] at (\xoffs+0, 0) {\includegraphics[width=0.33\linewidth]{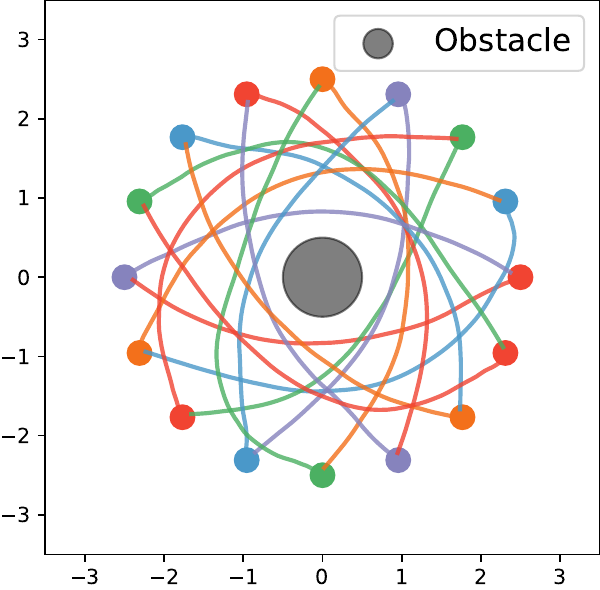}};
  \node[anchor=west] at (\xoffs+3.5, 0.0) {\includegraphics[width=0.4\linewidth]{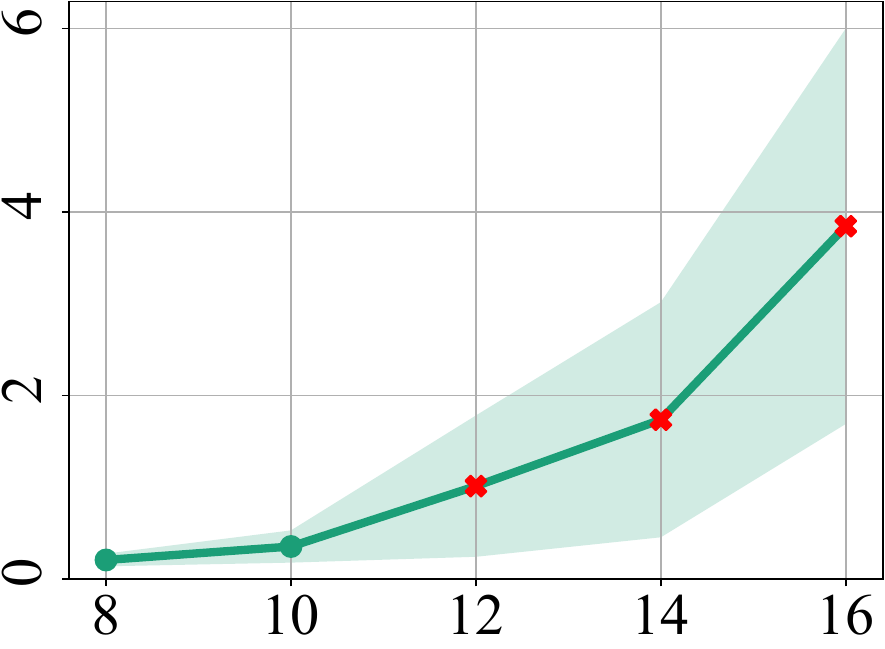}};
  \node[anchor=west,rotate=90] at (\xoffs+3.3, -0.5) {{\small Time [s]}};

  \node[anchor=west] at (0,-2.9) {{\small 1 Obst.}} ;
  \node[anchor=west] at (\xoffs+0, 1*\ystep) {\includegraphics[width=0.33\linewidth]{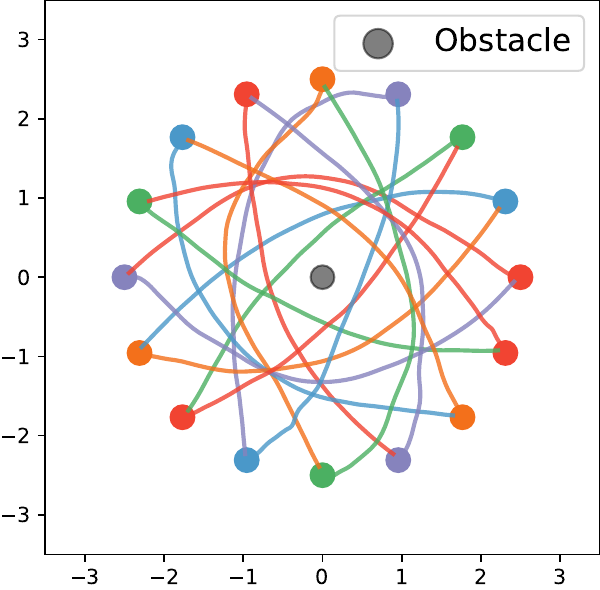}};
  \node[anchor=west] at (\xoffs+3.5, 1*\ystep){\includegraphics[width=0.4\linewidth]{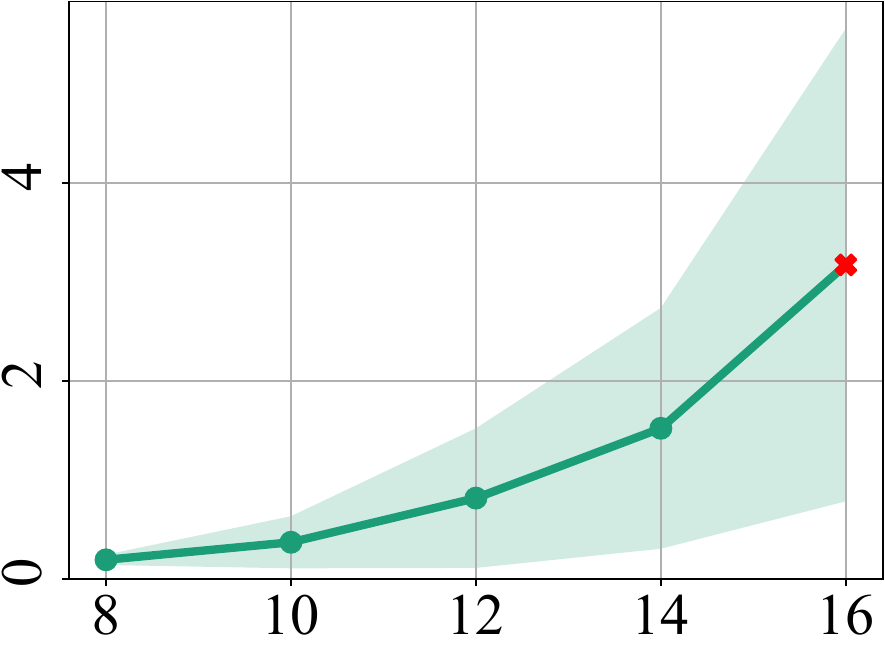}};
  \node[anchor=west,rotate=90] at (\xoffs+3.3, \ystep-0.5) {{\small Time [s]}};
  
  \node[anchor=west] at (0,-5.8) {{\small 2 Obst.}} ;
  \node[anchor=west] at (\xoffs+0, 2*\ystep) {\includegraphics[width=0.33\linewidth]{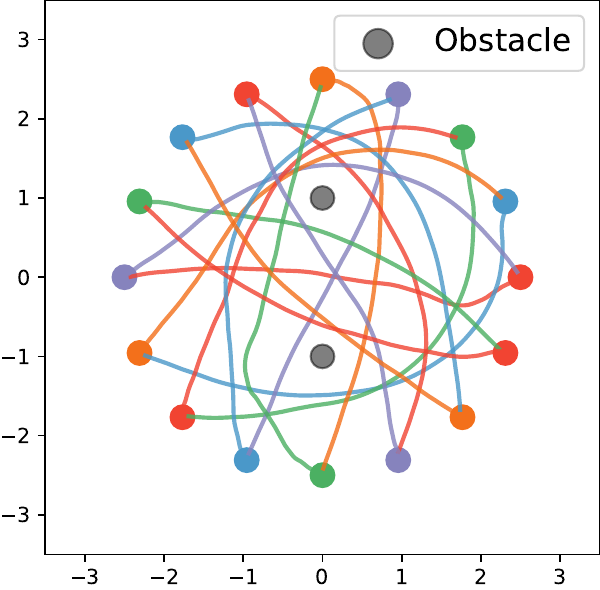}};
  \node[anchor=west] at (\xoffs+3.5, 2*\ystep) {\includegraphics[width=0.4\linewidth]{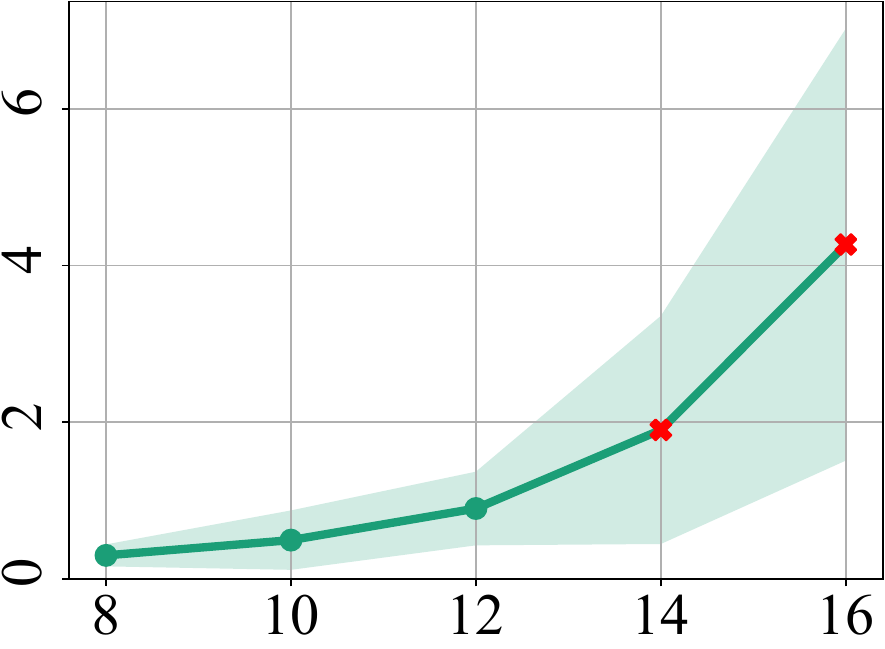}};
  \node[anchor=west,rotate=90] at (\xoffs+3.3, 2*\ystep-0.5) {{\small Time [s]}};
  
  \node[anchor=west] at (0,-8.8) {{\small 3 Obst.}} ;
  \node[anchor=west] at (\xoffs+0, 3*\ystep) {\includegraphics[width=0.33\linewidth]{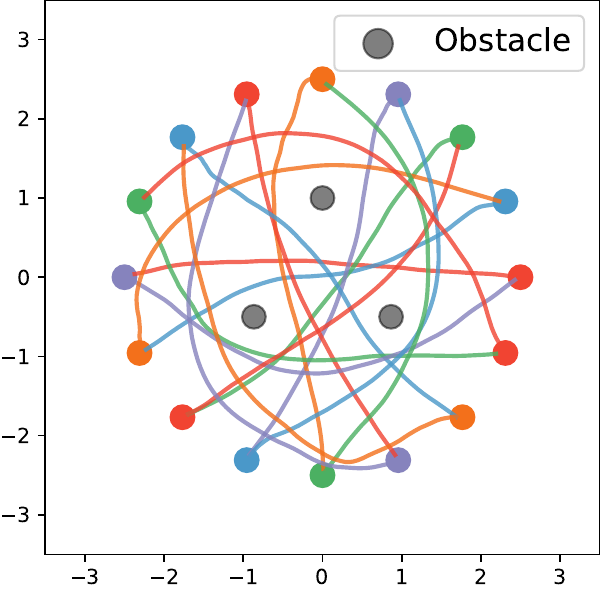}};
  \node[anchor=west] at (\xoffs+3.5, 3*\ystep) {\includegraphics[width=0.4\linewidth]{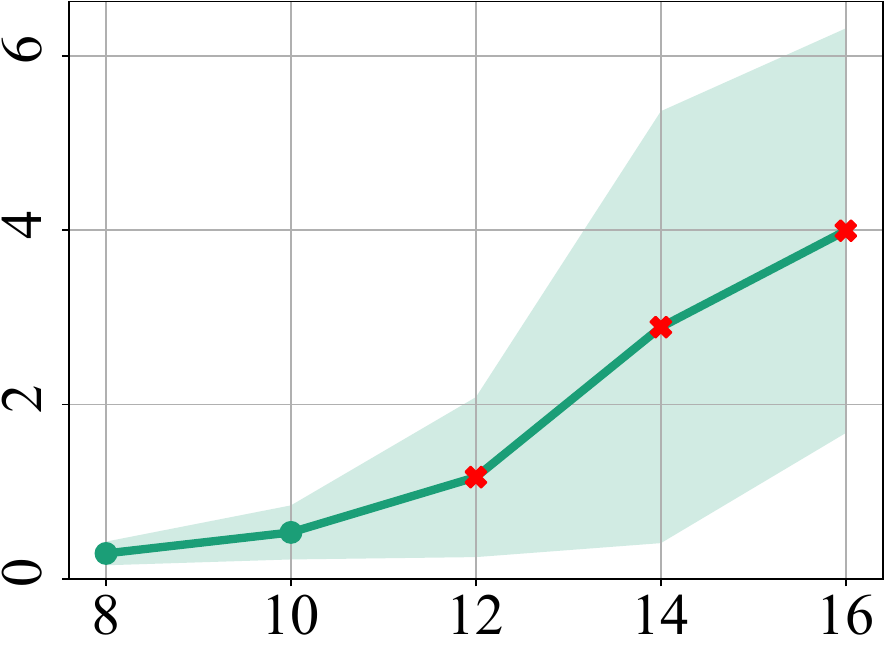}};
  \node[anchor=west,rotate=90] at (\xoffs+3.3, 3*\ystep-0.5) {{\small Time [s]}};
  
  \node[anchor=west] at (0,-11.8) {{\small 4 Obst.}} ;
  \node[anchor=west] at (\xoffs+0, 4*\ystep) {\includegraphics[width=0.33\linewidth]{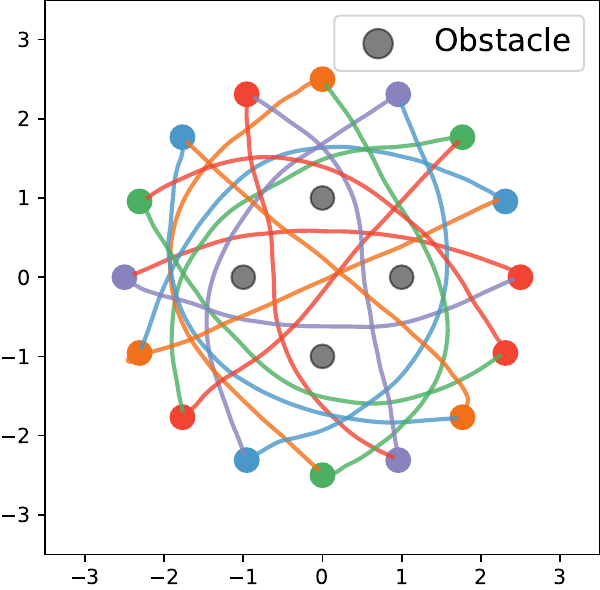}};
  \node[anchor=west] at (\xoffs+3.5, 4*\ystep) {\includegraphics[width=0.4\linewidth]{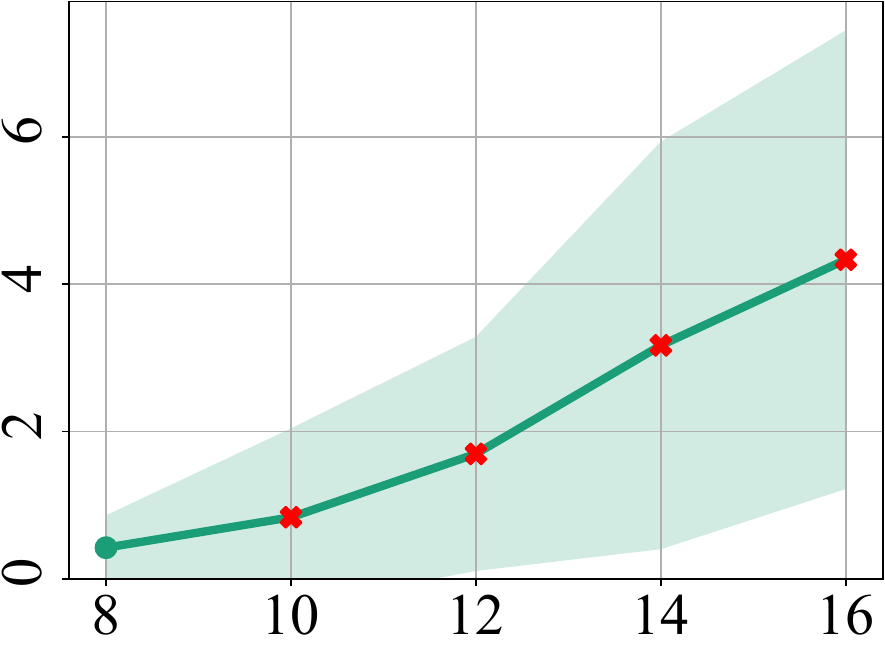}};
  \node[anchor=west,rotate=90] at (\xoffs+3.3, 4*\ystep-0.5) {{\small Time [s]}};
  \node[anchor=west] at (\xoffs+4.2, 4*\ystep-1.5) {{\small Number of Agents}};
  \node[anchor=west] at (0, -14){};
\end{tikzpicture}
\caption{Antipodal navigation scenarios for 16 robots with varying number of obstacles. The right-most column shows the computation time for finding initial solutions, averaged across 20 runs, excluding failed runs if any.}
\label{fig:obstacles}
\end{figure}
