# Supplementary material for: D4orm: Multi-Robot Trajectories with Dynamics-aware Diffusion Denoised Deformations
Source: arXiv:2503.12204 source file (2026-09-01)
Supplement: Supplementary file 2 [file recover.tex]

\begin{figure}[hp]
    \centering
    \begin{tikzpicture}
        \node[] at (0,0)
            {\includegraphics[width=0.6\columnwidth]
                {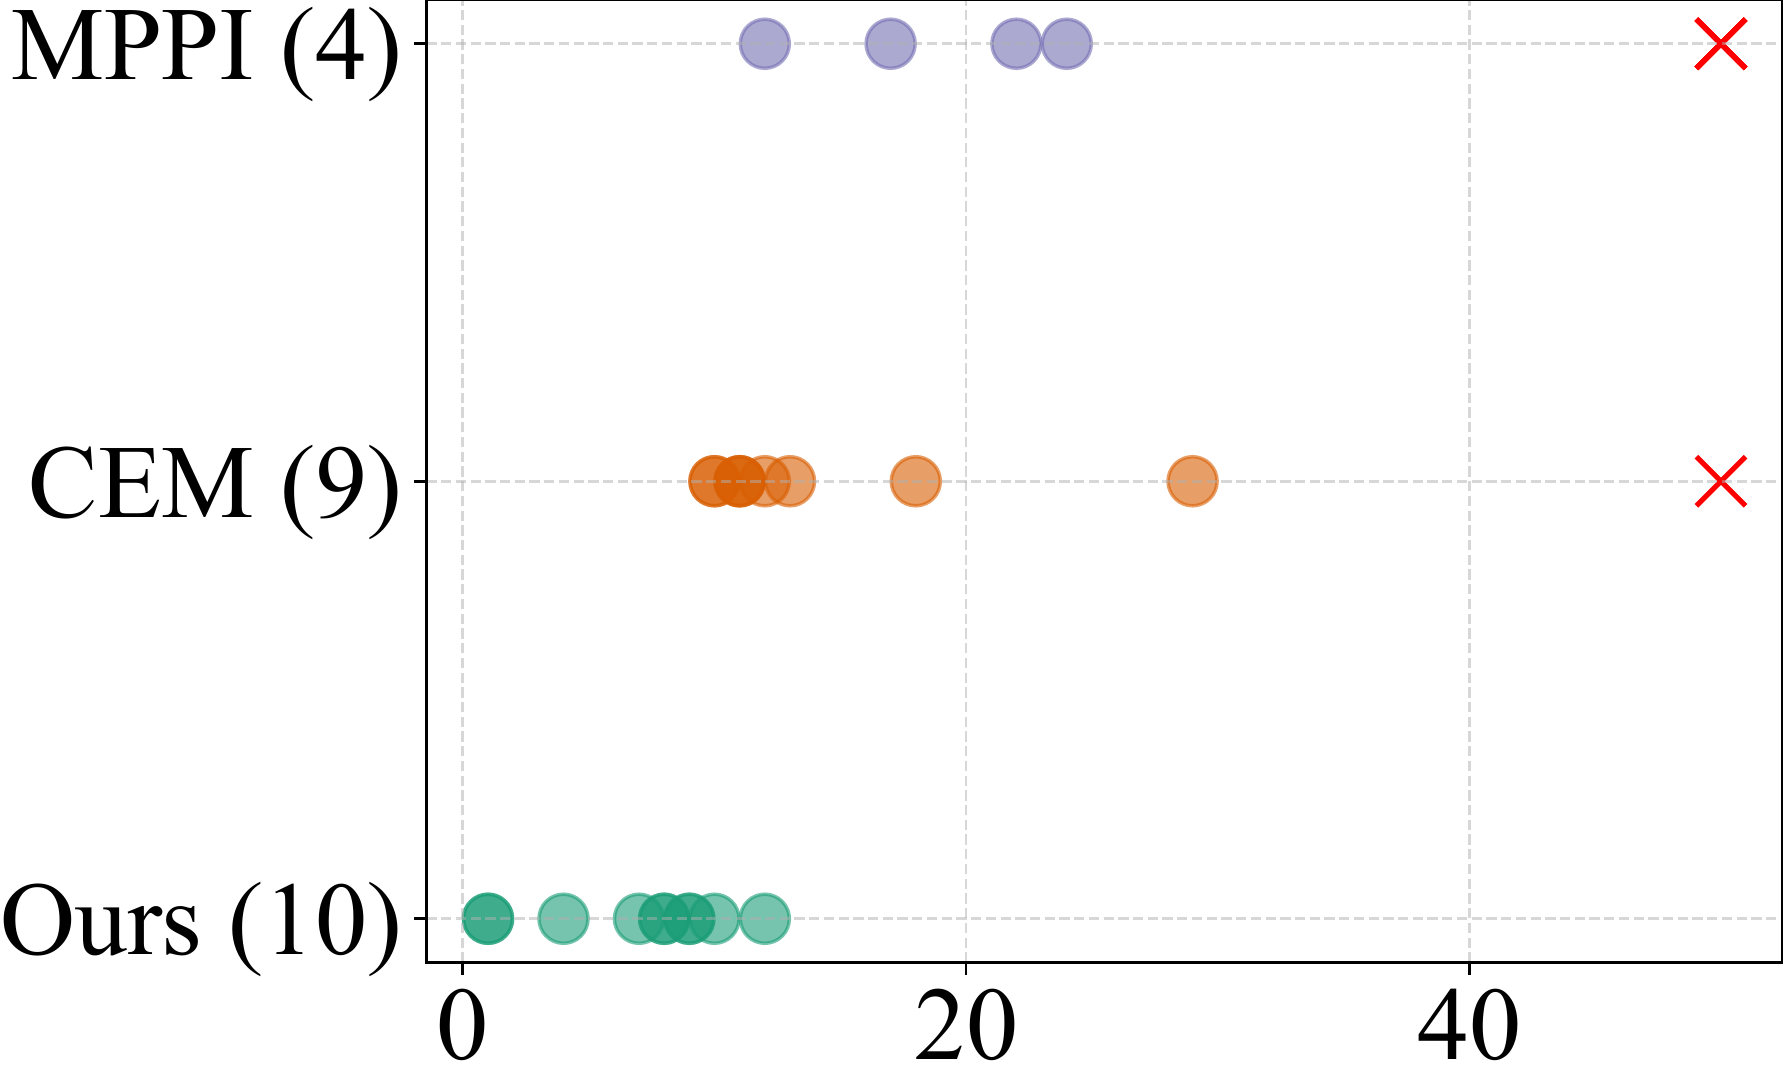}
            };
        \node[] at (0.5,-1.8)
            {{\small Number of Updates [$\times 10 ^ 2$]}};
    \end{tikzpicture}
    \caption{Recovering from a local optimum for 10 initial conditions. All methods are given the same high-reward (though incorrect) initial solutions. A colored dot indicates that the method is able to recover (the number in parenthesis indicates the success count), while {\textcolor{red}{$\times$}} indicates failure at timeout. }
    \label{fig:recover}
\end{figure}
